# Supplementary material for: 3DCaricShop: A Dataset and A Baseline Method for Single-view 3D Caricature Face Reconstruction
Source: arXiv:2103.08204 source file (2021-03-15)
Supplement: Supplementary file 1 [file Corrections.tex]

\section{Typos Correction}
\label{sec:corrections}
After a careful examination, we correct 2 typos in our submission as following:
\begin{itemize}
    \vspace{-1mm}
    \item For equation (1) in Sec 4.1, $\mathbf{F}$ represents the front view normal map and $\mathbf{B}$ is the back view one.
    \vspace{-1mm}
    \item The caption of Figure 9 should be `(a) input; (b) GT; (c) NICP w/o landmark; (d) NICP w/o PCA projection; (d) ours'.
\end{itemize}
